# Supplementary material for: Detecting ADS-B Spoofing Attacks using Deep Neural Networks
Source: arXiv:1904.09969 source file (2019-04-22)
Supplement: Supplementary file 1 [file appendices.tex]

\newpage
\appendix

\subsection{Simulate Transmit Frequency Offset in IQ Samples}
Each ADS-B message consists of $8\mu$s preamble and $112 \mu$s data block (112 bits in total). 
There are a total of $m=120$ pulses with different time positions to encode the information to be transmitted (i.e., Manchester coding). 
Hence, the transmitted passband signal $s_p(t)$ can be represented as follows \cite{leonardi2017air, madhow2008fundamentals}:
\begin{equation}
    s_p(t) = Re[\sqrt{2} s(t) e^{j 2 \pi f_c t}]
\end{equation}
where 
\begin{equation}
    s(t) = \left[ \sum_{m=1}^{120} rect\left( \frac{t-2mT+c_mT + T/2}{T} \right) \right],
\end{equation}
is the baseband signal with a phase of zero. 
In general, we have $s(t)=s_c(t) + j s_s(t)$ and $s_p(t) = e(t) \cos (2\pi f_c t + \theta(t))$, where $e(t)=|s(t)|=\sqrt{s_c^2(t) + s_s^2(t)}$ is the envelope and $\theta(t)=\tan^{-1} \frac{s_c(t)}{s_s(t)}$ is the phase.

In order to generate IQ samples that can be transmitted by the USRP, we first sample $s(t)$ with a sampling rate of $1/T_s$ where $T_s=T/2 =0.2\mu$s and obtain $s[k]=s(kT_s)$.  
Hence, each ADS-B message is represented by $\{s[k]\}$ with a total of $240$ samples.
After that, we generate one I sample and one Q sample for each $s[k]$.
%that have the same magnitude  and a phase of zero. 
IQ samples are then stored in the binary format as interleaving unsigned bytes.

In the presence of a transmit frequency offset $\Delta f$, the transmitted signal with the embedded Doppler shift becomes
\begin{align}
    s_p(t) &= Re[\sqrt{2} s(t) e^{j 2 \pi (f_c + \Delta f) t}] \\
    &= Re[(\sqrt{2}s(t) e^{j 2 \pi \Delta f t}) e^{j 2 \pi f_c t}].
\end{align}
Hence, in order to simulate the transmit freqeuency offset, we can introduce a phase change in the transmitted signal by multiplying each complex sample  by $e^{j 2 \pi \Delta f t}$, where $t=kT_s$. 

\subsection{Simulate Doppler Shift}
Let the baseband signal be $s(t)$ and its passband signal at a center frequency of $f_c$ be $s_p(t)=Re[\sqrt{2}s(t)e^{j2\pi f_c t}]$. 
Let their Fourier transform be $S(f)$ and $S_p(f)$, respectively. 
The relationship between $S(f)$ and $S_p(f)$ is 
\begin{equation}
    S(f) = \sqrt{2} S_p^+ (f+f_c),
\end{equation}
where $S_p^+(f)$ is the segment of $S_p(f)$ occupying positive frequencies. 

Due to the Doppler shift, the observed frequency $f_o$ is 
\begin{equation}
    f_o = \left(\frac{c+v_o}{c-v_s} \right) f = (1 + \alpha) f,
\end{equation}
where $\alpha = \frac{c+v_o}{c-v_s} - 1$. 
As a result, the observed passband signal becomes 
\begin{equation}
    S_p'(f) = S_p \left(\frac{1}{1+\alpha} f \right).
\end{equation}
Hence, we have 
\begin{align}
    s'_p(t) &= (1+\alpha) s_p((1+\alpha) t) \\
    &=(1+\alpha) Re[\sqrt{2} s((1+\alpha)t) e^{j 2\pi  f_c (1+\alpha) t}]. 
\end{align}

For example, if $s_p(t) = \cos(2\pi f_c t)$ and $f_d=(1+\alpha) f_c$, then we have $s_p'(t) = \cos(2\pi f_d t) = s_p((1+\alpha) t)$. 

Note that since the bandwidth of ADS-B signal is about 50 kHz, it can be considered as a narrowband signal, as compared to the center frequency of 1090 MHz. 
As a result, the Doppler effect essentially results in a frequency shift \cite{matz2011fundamentals}.
